# Supplementary material for: Worse than Random? An Embarrassingly Simple Probing Evaluation of Large Multimodal Models in Medical VQA
Source: arXiv:2405.20421 source file (2025-06-10)
Supplement: Supplementary file 1 [file benchmark_detail.tex]

\section{Benchmark Details}
This appendix provides a comprehensive overview of the MMIR benchmark. It details the dataset curation process, including error category definitions, the synthetic inconsistency generation mechanism, the auto‐verification and human validation processes, and the task prompts for evaluation. These details are intended to facilitate reproducibility and provide clarity on the inner workings of MMIR.

\subsection{Inconsistency Error Category Definitions}
\label{appendix:sec:error category}

The MMIR benchmark employs five pre-defined error categories. These categories are designed based on semantic guidelines so that the generator model can propose diverse and generalizable inconsistencies without being tied to any specific artifact type.

\begin{itemize}
    \item \textbf{A. Factual Contradiction} 
    
    Direct conflict between two or more elements (text–text, text–image, or image–image) within the modified content.
    
    \emph{Example (Text–Text): The product title says “Caffeinated,” while the description states “Caffeine-free.”\\Example (Text–Image): The image shows a green tea bag, but the accompanying text describes a “fruit infusion.”}

    \item \textbf{B. Identity Misattribution} 
    
    Mislabeling of entities (objects, locations, brands, people) that conflict with other elements.
    
    \emph{Example: A product lists “Country of Origin: China” while the manufacturer is described as “Elmwood Inn (USA).”}

    \item \textbf{C. Contextual Mismatch} 
    
    Tonal, thematic, or situational incompatibility between elements.
    
    \emph{Example: A celebratory image of diplomats shaking hands is paired with an article about violent clashes.}

    \item \textbf{D. Quantitative Discrepancy} 
    
    Numerical or statistical inconsistencies between elements.
    
    \emph{Example: A graph labeled “50\% growth” shows flat bars.}

    \item \textbf{E. Temporal/Spatial Incoherence} 
    
    Implied timelines, dates, or spatial relationships that are impossible or conflicting.
    
    \emph{Example: A map labeled “North America” depicts landmarks from Europe.}
\end{itemize}

These definitions serve as guidelines during the synthetic inconsistency generation process, ensuring that the proposed errors are semantically meaningful and cover a broad spectrum of potential real-world mistakes.

\subsection{Generator Model and Self-Evaluation Loop}
\label{appendix:sec:generator}

\subsubsection{Generator Model Prompt}

To create adversarial examples, the generator model (o1, 1217) is provided with rich context consisting of the annotated artifact $A_i^{\text{SOM}}$ and its set of elements $E_i$. The task prompt includes detailed instructions regarding the types of modifications to propose, along with the following guidelines:

\begin{itemize}
    \item \textbf{Modification Format:} Each modification must be expressed as: 

    ```Modify [id] [original\_content] [new\_content]```

    For image fields, the original content includes the full details (e.g., URL), and the new content is a caption starting with "Image, description: ". For text fields, the new content should be of similar length to the original.

    \item \textbf{Error Categories:} The generator must propose one modification per error category. If it cannot propose an inconsistency for a given category, it may skip that category.
\end{itemize}

The generator output is structured as:

$$P_m=\left\{\text { edit }_m, \mathrm{GT}_m, \text { category }{ }_m, \text { rationale }_m\right\}$$

where the ground-truth $\mathrm{GT}_m$ is defined as:

$$\mathrm{GT}_m \in\left\{\mathrm{id}_j\right\} \cup\left\{\left(\mathrm{id}_j, \mathrm{id}_k\right) \mid j \neq k\right\}$$

indicating either a single-element ID (for single-element inconsistencies) or a pair of distinct element IDs (for relational inconsistencies).

\subsubsection{Self-Evaluation Loop}
We follow a generator-evaluator loop that refines proposals through iterative self-assessment. A simplified Python snippet of the loop function is provided below:

\begin{lstlisting}
def loop(client, image_dir, frame_id, task: str, evaluator_prompt: str, generator_prompt: str) -> tuple[str, list[dict]]:
    """Keep generating and evaluating until requirements are met."""
    memory = []
    chain_of_thought = []
    
    thoughts, result = generate(client, image_dir, frame_id, generator_prompt, task)
    memory.append(result)
    chain_of_thought.append({"thoughts": thoughts, "result": result})
    
    loop_count = 1
    while True:
        all_pass = True
        evaluation, feedback = evaluate(client, image_dir, frame_id, evaluator_prompt, result, task)
        for eval_line in evaluation.split("\n"):
            if eval_line.strip() != "PASS":
                all_pass = False
                break
        if all_pass or loop_count == 2:
            return result, evaluation
            
        context = "\n".join([
            "Previous attempts:",
            *[f"- {m}" for m in memory],
            f"\nFeedback: {feedback}"
        ])
        thoughts, result = generate(client, image_dir, frame_id, generator_prompt, task, context)
        memory.append(result)
        chain_of_thought.append({"thoughts": thoughts, "result": result})
        loop_count += 1
\end{lstlisting}

In this loop, the generator produces proposals which are then evaluated against the following criteria (as specified in the evaluator prompt):
\begin{itemize}
    \item \textbf{Category Compliance:} The edit must match the intended error category.
    \item \textbf{Atomic Modification:} Exactly one inconsistency should be introduced.
    \item \textbf{Visual Consistency:} The modified screenshot must visibly reflect the error without relying on external context.
    \item \textbf{Element Validity:} The referenced element IDs must exist in the artifact.
\end{itemize}

Only proposals receiving a "PASS" in the evaluation are retained. The loop iterates until either all criteria are met or a maximum of two iterations is reached.

\subsubsection{Prompt details for generator-evaluator proposal generation framework}
\begin{lstlisting}
    evaluator_prompt = """
Evaluate the following proposals one by one for:
1. Category Compliance: Introduced inconsistency matches the category definition (A-E)
2. Atomic Modification: Introduce EXACTLY ONE inconsistency without side effects
3. Visual Consistency: Conflict visible in the modified screenshot (with NO reliance on original page knowledge or external context)
4. Element Validity: Conflict IDs exist in observations

You should be evaluating only and not attemping to solve the task.
For each proposal, only output "PASS" if all criteria are met and you have no further suggestions for improvements.
Output your evaluation concisely in the following format.

<evaluation>
PASS, NEEDS_IMPROVEMENT, or FAIL <-- For each proposal
</evaluation>
<feedback>
What needs improvement and why. <-- For proposals that need improvement
</feedback>
"""

    generator_prompt = """
Your goal is to complete the task based on <user input>. If there are feedback 
from your previous generations, you should reflect on them to improve proposals that NEEDS_IMPROVEMENT or FAIL. Leave the PASS proposals as they are. 

Output your answer concisely in the following format: 

<thoughts>
[Your understanding of the task and feedback and how you plan to improve]
</thoughts>

<response>
[Your response here]
</response>
"""

    task_prompt = f"""
<user input>
Your task is to modify a {category_str} to create inconsistency. For each given category of inconsistency, you will propose a modification action that introduces the inconsistency in the modified {category_str}.
    
Here's the information you'll have:
Screenshot of the urrent {category_str}: This is a screenshot of the {category_str}, with each editable element assigned a unique numerical id. Each bounding box and its respective id share the same color.
The Observation, which lists the IDs of all editable elements on the current {category_str} with their content, in the format [id] [tagType] [content], separated by "\n". Each id is mapped with the id in the screenshot. tagType is the type of the element, such as button, link, or textbox. For example, "[21] [SPAN] [Add to Wish List]" means that there is a span with id 21 and text content 'Add to Wish List' on the current {category_str}. "[23] [IMG] [Image, description: a beige powder on a white background, url: http://localhost:7770/media/catalog/product/cache/829a59e57f886f8cf0598ffca4f8a940/B/0/B074DBMG66.0.jpg]" means that there is an image on the current screen with id 23, with a description of the image and its url specified.

Here are the categories of errors you can introduce:
A. Factual Contradiction -  Direct conflict between two or more elements (text-text, text-image, or image-image). For example, The product title says "Caffeinated," while the description states "Caffeine-free." Another example: The image shows a green tea bag, but the text describes a "fruit infusion."
B. Identity Misattribution - Mislabeling of entities (objects, locations, brands, people) that conflict with other elements. Example: Product "Country of Origin: China" contradicts manufacturer info "Elmwood Inn (USA)."
C. Contextual Mismatch - Tonal, thematic, or situational incompatibility between elements. Example: A celebratory image of diplomats shaking hands paired with an article about violent clashes.
D. Quantitative Discrepancy - Numerical or statistical inconsistencies between elements. Example: A graph labeled "50%\ growth" shows flat bars.
E. Temporal/Spatial Incoherence - Implied timelines, dates, or spatial relationships that are impossible or conflicting. Example: A map labeled "North America" depicts landmarks from Europe

Here are the rules for the modification action:
The modification action you can propose to introduce inconsistency must be in the format of "Modify [id] [original_content] [new_content]": This action proposes to edit the orignal field assigned with the id to the new content to introduce inconsistency. If you propose to modify an image field, the [original_content] field should include the full content from observation including the url; the [new_content] field should be a caption describing the updated image, starting with "Image, description: ", no url needed. If you propose to modify a text field, the new content string should be about the same length as the original text field. For each inconsistency category, you should try to propose a modification action that introduces an inconsistency in that category. If you can't find a way to introduce an inconsistency in a category, you can skip it. Prioritize proposing edits on text fields over image fields.

Generate the response in the correct format. For each inconsistency, the format should be:
<proposal>
  <cat>[A-E]</cat> <-- Category letter
  <ele>[ID1,ID2]</ele> <-- Conflicting element IDs
  <mod>Modify [ID] [Original Content] [New Content]</mod> <-- Modification plan
  <rationale>Visible conflict explanation</rationale> <-- Visual verification
</proposal>
</user input>
"""
\end{lstlisting}

\subsection{Auto-Verification and Editing Process}
\label{appendix:sec:verifier and editor}

Following proposal generation, an auto-verification step filters the proposals based on format and backend constraints. Specifically:

\begin{itemize}
    \item \textbf{Edit Format Verification:} The system uses a regular expression to ensure that each proposed edit adheres to the required format: "Modify [id] [old\_content] [new\_content]".

    \item \textbf{Element Matching:} For web-sourced artifacts, the proposal’s element ID is used to locate the corresponding element and its bounding box in the metadata. The system checks that both the content and bounding box match an editable element in the HTML/PPTX structure. For image edits, the new content (a caption) is cross-referenced against an MSCOCO image database to verify its appropriateness.

    Proposals that pass these checks are automatically saved for further processing.
    
\end{itemize}

For web pages, we use the CDP to perform edit:

\begin{lstlisting}
# text edit
client.send(
    "Runtime.callFunctionOn",
    {
        "objectId": object_id, 
        "functionDeclaration": f"function() {{ this.nodeValue = '{new_content}'; }}",
        "arguments": [],
        "returnByValue": True
    }
)
# image edit
with open(new_content, "rb") as image_file:
    img = Image.open(image_file)
    new_image_width, new_image_height = img.size  # get original width and height for resizing
    aspect_ratio = new_image_width / new_image_height
    if w / h > aspect_ratio:
        w, h = w, int(w / aspect_ratio)
    else:
        w, h = int(h * aspect_ratio), h
    img = img.resize((w, h), Image.Resampling.LANCZOS)
    buffer = BytesIO()
    img.save(buffer, format="JPEG")
    buffer.seek(0)
    base64_image = base64.b64encode(buffer.read()).decode("utf-8")
    new_image = f"data:image/jpeg;base64,{base64_image}"
client.send(
    "Runtime.callFunctionOn",
    {
        "objectId": object_id,
        "functionDeclaration": f"""
            function() {{
                this.src = '{new_image}';
            }}
            """,
        "arguments": [],
        "returnByValue": True
    }
)
\end{lstlisting}

For Zenodo presentation, we use the \texttt{python-pptx} library:

\begin{lstlisting}
# text edit
if target_shape.has_text_frame: # text edit
    text_frame = target_shape.text_frame
    for paragraph in text_frame.paragraphs:
        for run in paragraph.runs:
            if edit_info["old_content"] in run.text:
                try:
                    run.text = run.text.replace(edit_info["old_content"], edit_info["new_content"])
                    success = True
                    break
                except:
                    success = False
# image edit
left, top, orig_width, orig_height = target_shape.left, target_shape.top, target_shape.width, target_shape.height
pic = target_shape._element
pic.getparent().remove(pic)
new_image_path = f"{coco_image_dir}/{edit_info['new_img_path']}"
with Image.open(new_image_path) as img:
    new_width, new_height = img.size
new_aspect = new_width / new_height
orig_aspect = orig_width / orig_height
if new_aspect > orig_aspect:
    scaled_width = orig_width
    scaled_height = int(scaled_width / new_aspect)
else:
    scaled_height = orig_height
    scaled_width = int(scaled_height * new_aspect)
new_left = left + (orig_width - scaled_width) // 2
new_top = top + (orig_height - scaled_height) // 2
try:
    slide.shapes.add_picture(  # Add the new image in the same location and size
        new_image_path, new_left, new_top, scaled_width, scaled_height
    )
    success = True
except:
    success = False
\end{lstlisting}
