# Supplementary material for: Worse than Random? An Embarrassingly Simple Probing Evaluation of Large Multimodal Models in Medical VQA
Source: arXiv:2405.20421 source file (2025-06-10)
Supplement: Supplementary file 2 [file ablation_cot_som.tex]

\begin{table}[t]
% \small
\caption{\textbf{Probing analysis on the affect of different prompting methods on MLLMs' performance. Performance under different probing settings is compared with the vanilla setting.} Gains are in blue and drops are in red.
}
\begin{center}
\vspace{-10pt}
\resizebox{\linewidth}{!}{
\begin{tabular}{lccccc}
\toprule

Models & Vanilla & + CoT & + SoM & + Both & MM-CoT\\
\midrule
\multicolumn{6}{>{\columncolor{gray!15}}l}{\textit{Proprietary Models}}\\
o1 (1217)           & 51.40  & -- & \textcolor{red}{-0.66}  & -- & \textcolor{blue}{+0.09}\\
GPT-4o (1120)       & 33.14  & -- & \textcolor{blue}{+5.34} & -- & \textcolor{blue}{+4.40}\\
\multicolumn{6}{>{\columncolor{gray!15}}l}{\textit{Open-sourced Models}}\\
Qwen2.5-VL-7B       & 17.60 & \textcolor{blue}{+0.28} & \textcolor{blue}{+0.09} & \textcolor{blue}{+0.28} &\\ 
LLaVA-NeXT-7B       & 14.70 & \textcolor{red}{-1.78}  & \textcolor{red}{-2.53} & \textcolor{red}{-0.47} & \\
InternVL2.5-8B      & 14.23 & \textcolor{blue}{+2.24} & \textcolor{red}{-0.66} & \textcolor{red}{-1.41} & \\
Phi-3.5-Vision-4B   & 14.23 & \textcolor{red}{-0.38}  & \textcolor{blue}{+0.47} & \textcolor{blue}{+0.84} & \\
\bottomrule
\end{tabular}
}
\end{center}
\vspace{-10pt}
\label{tab:ablation_cot_som}
\end{table}
